# Supplementary material for: Likelihood-based inference and forecasting for trawl processes: a stochastic optimization approach
Source: arXiv:2308.16092 source file (2023-08-30)
Supplement: Supplementary file 1 [file Simple_ambit_field_inference.tex]

\subsection{Simple ambit fields inference}\label{subsection:simple_ambit_field}
Trawl processes are stationary and infinitely divisible continuous-time stochastic processes which can describe a wide range of possible serial correlation patterns in data. A direct generalization of the trawl process to spatio-temporal fields is given by the ambit field $Y$ with
\begin{equation}
    Y_t(\mathbf{x}) = \int_{A_t(\mathbf{x})} K_{t,\mathbf{x}}\left(\bar{t},\bar{\mathbf{x}}\right) \sigma(\bar{t},\bar{\mathbf{x}}) L(\mathrm{d}\bar{t},\mathrm{d}\bar{\mathbf{x}}),\label{def:ambit_fields}
\end{equation}
where the deterministic kernel $K$ multiplied by the volatility $\sigma$ is integrated against the L\'evy basis $L$ and where $A_t(\mathbf{x}) \in \R^{d+1}$ is a collection of time and space-indexed sets. The integration is understood in the sense of \cite[Theorem 2.7]{rajput1989spectral} when the integrand is determinstic, i.e.~$\sigma = 1$, and in the sense of 
\cite{walsh,bichteler1983random} and \cite{kluppelberg} for stochastic $\sigma$. Ambit fields provide a powerful statistical modelling framework, and we only mention a few examples.  \cite{di2014forecasting} uses Gaussian L\'evy bases to forecast 
energy market contracts and 
\cite{ambit_book} discusses forward curve modelling by ambit fields in Chapter $11$. \cite{emil_h_phd_thesis} provides extensive analyses of turbulence and energy dissipation through  L\'evy modelling and ambit fields and \cite{jonsdottir2008levy} introduces a new approach by ambit fields to growth modelling and applies it to tumour growth. The last two papers use GMM to calibrate the model parameters, which can have poor finite sample performance or be unfeasible for somedistributions (e.g.~see page $15$ of \citep{emil_h_phd_thesis}). \cite{jonsdottir2008levy} introduces non-rectangular ambit sets and non-Gaussian L\'evy bases, extending beyond both the Markovian and Gaussian frameworks for spatio-temporal modelling. This added complexity of the model which helps replicate the stylised statistical facts of the datasets is also the issue with applying these models further. For example, we are not aware of deterministic or probabilistic forecasting formulae for ambit fields, even in the case when $\sigma = 1 $ in \eqref{def:ambit_fields}. To improve on this, we propose the use of simple ambit fields, which we discuss below.

Simple ambit fields are a natural extension of trawl processes to spatio-temporal fields and are given by 
$Y_t(\mathbf{x}) = L(A_t(\mathbf{x}))$. Similarly to trawl processes, simple ambit fields provide a rich class of infinitely divisible stochastic processes with flexible spatio-temporal autocorrelation structures and marginal distributions, which can be modelled independently one of the other. In particular, the autocovariance and autocorrelation structures are 
\begin{align*}
\Cov(Y_{t_1}(\mathbf{x}_1),Y_{t_2}(\mathbf{x}_2)) &=  \mathrm{Leb}\left(A_{t_1}(\mathbf{x})\cap A_{t_2}(\mathbf{x}_2)\right)  \Var(L^{'})\\ \Corr(Y_{t_1}(\mathbf{x}_1),Y_{t_2}(\mathbf{x}_2)) &= \mathrm{Leb}\left((A_{t_1}(\mathbf{x}_1)\cap A_{t_2}(\mathbf{x}_2)\right) / \, {\mathrm{Leb}\left(A\right)} 
 \end{align*}
and $Y$ can have any infinitely divisible distribution. We generally fix an ambit set $A \in \R^{d+1}$ and let $A_t(\mathbf{x}) = A + (t,\mathbf{x})$ be the set translation of $A$. With this choice of ambit sets, $Y$ is stationary and can be simulated efficiently by two algorithms (see Section $5$ of \cite{leonte2022simulation_arxiv}). Further, we show that both the composite likelihood inference and forecasting methodology extends from trawl processes to simple ambit fields, making the latter a tractable approach for spatio-temporal statistics. To begin with, the following conditional mean forecast formula holds.
\begin{theorem}Assume that the L\'evy seed $L^{'}$ is integrable. Then 
\begin{equation*}
    \ev\left[Y_{t+\Delta_t}(\mathbf{x}+ \mathbf{\Delta_x}) | Y_t(\mathbf{x}) \right] = \rho \, Y_t(\mathbf{x}) + (1-\rho) \,\ev[Y_t(\mathbf{x})],
\end{equation*}
where 
\begin{equation*}
\rho\ =  \frac{\mathrm{Leb}\left(A_t(\mathbf{x}) \cap A_{t+\Delta_t}(\mathbf{x} + \mathbf{\Delta_x})\right)}{\mathrm{Leb}(A)}.
\end{equation*}
\end{theorem}
The same proof as for Theorem \ref{thm:non_markovian_forecast} applies and probabilistic sampling can be performed as described in Section \ref{section_forecasting}. We now turn our attention to composite likelihood estimation. For ease of exposition, we present the theory in $d=1$ dimensions.

Let $\tau,\,  x>0$ and assume we observe a realization $\mathbf{y}$ of the simple ambit field $Y$ at time-space coordinates $\{(i\tau,jx): 1 \le i \le n_s, 1 \le j \le n_x\}$. Then $\y$ is $n_s \times n_t$ dimensional. Define the temporal and spatial pairwise likelihood function at lags $k_t$ and $k_s$ by
\begin{align*}
    {PL}_{\textrm{t}}^{k_t}(\bt;\y) &= \prod_{i=1}^{n_t-k_t} 
 \prod_{j=1}^{n_s}p\left(y_{i\tau}(jx),y_{(i+k_t)\tau}(jx);\bt\right),     \\
     {PL}_{\textrm{s}}^{k_s}(\bt;\y)& = \prod_{i=1}^{n_t} 
 \prod_{j=1}^{n_s-k_s}p\left(y_{i\tau}(jx),y_{i\tau}\left((j+k_s)x\right);\bt\right), 
\end{align*}
and the pairwise likelihood function by
\begin{equation*}
\mathcal{L}_{PL}(\bt) =  \prod_{k_t \in K_t} \prod_{k_s \in K_s} {PL}_{\textrm{t}}^{k_t}(\bt;\y)   \, {PL}_{\textrm{s}}^{k_s}(\bt;\y),
\end{equation*}
where $K_t$ and $K_s$ are the numbers of temporal, respectively spatial lags to be included. The PL estimator is then given by
\begin{equation*}
\end{equation*}
\begin{equation*}
    \hat{\bt}^{PL} \defeq \argmax_{\bt} \mathcal{L}_{PL}(\bt).
\end{equation*}
The pairwise likelihoods can be estimated with samples, as described at the beginning of Section \ref{subsection:trawl_inference_as_a_stoch_optim_problem}. The variance reductions techniques presented in Subsections \ref{subsubsection:pg}, \ref{subsubsection_linear_control_variateas} and in S\ref{supplementary:measure_valued_grad}, i.e.~pathwise gradients, measure-value gradients and control variates can be applied directly, with no change. 

[some tables with results to add]

\textbf{Further research}

Firstly, the above composite likelihood inference procedure for simple ambit fields only included pairs corresponding to either vertical or horizontal translations of ambit sets. Given an $n_s \times n_t$ matrix $\y$ of observations, these pairs only account for a fraction of the total number of pairs for which the corresponding ambit sets have non-empty intersection. We expect that using more pairs will result in better finite sample properties of our estimators. The difficulty lies in approximating the areas of the intersections of ambit sets which are translated along both axes of coordinates. A solution would be to work with families of trawl functions $\phi$ for which these areas are available analytically.

Secondly, although composite likelihood proves to be an efficient inference method for simple ambit fields, it can not be applied to ambit fields in general. The presence of the deterministic kernel $K$ or stochastic volatility $\sigma$ in \ref{def:ambit_fields} makes the pairwise likelihood and even the marginal likelihood function intractable. It is not clear if ambit fields are always ergodic and further and even so, GMM is known to perform poorly for certain distributions (e.g.~NIG). This significantly restricts parameter calibration and the applicability of ambit fields to real-world modelling problems. Nevertheless, using ambit fields instead of simple ambit fields has advantages, e.g.~directly modelling non-stationary behaviour by ambit fields rather then fitting simple ambit fields to a de-trended and de-seasonalised dataset, which might be only covariance stationary and not strictly stationary. To this extent, we refer the new advances in the amortized likelihood inference \cite{?} [ a few citations], which use first use neural networks to approximate the likelihood function and then perform MCMC to sample from the posterior distribution of the model parameters.
